# Supplementary material for: QAMPARI: An Open-domain Question Answering Benchmark for Questions with Many Answers from Multiple Paragraphs
Source: arXiv:2205.12665 source file (2023-05-29)
Supplement: Supplementary file 1 [file appendix_H.tex]

\section{Additional statistics}
\label{sec:first_word_stats}

The 8 most common first words for these sets are: What 36.6\%, Who 21.9\%, Which
19.1\%, Where 3\%, In 2.3\%, The 1.8\%, For 1\%, From 0.3\%. There are in total 236 different first words for our validation and test set questions.
